# Supplementary material for: Time to Reason: Scalable Neurosymbolic Learning for LTLf via Fuzzy Semantics
Source: arXiv:2608.16443 source file (2026-08-17)
Supplement: Supplementary file 1 [file appendixB.tex]

\section{Statistical Tests}
\label{app2}

% \begin{table*}[ht]
% \centering
% \caption{\riccardo{TEMPORARY TABLE: Experiments with formula "((!y1 U x0) \& (!z3 U y2))", varying the sequence length. No statistical tests performed yet. Some runs of \NeSyA are yet to be completed (marked in yellow)} }
% \resizebox{\textwidth}{!}{
% \begin{tabular}{c ccc ccc ccc}
% \toprule
% & \multicolumn{3}{c}{\textbf{Img. Acc.} ($\% \uparrow$)} & \multicolumn{3}{c}{\textbf{Seq. Acc.} ($\% \uparrow$)} & \multicolumn{3}{c}{\textbf{Time} (s $\downarrow$)} \\
% \cmidrule(lr){2-4} \cmidrule(lr){5-7} \cmidrule(lr){8-10}
% Len & \TILR & \FuzzyDFA & \NeSyA & \TILR & \FuzzyDFA & \NeSyA & \TILR & \FuzzyDFA & \NeSyA \\
% \midrule
% 20 & 98.2 & 98.2 & 98.2 & \textbf{97.7} & 97.3 & 97.7 & \textbf{0.04} & 0.34 & 0.33 \\
% 40 & 98.1 & 98.1 & 98.1 & 98.5 & 98.2 & \textbf{98.6} & \textbf{0.09} & 0.59 & 0.61 \\
% 60 & 98.0 & 97.9 & 98.0 & \textbf{98.3} & \textbf{98.3} & 98.2 & \textbf{0.12} & 0.87 & 0.93 \\
% 80 & 98.2 & 98.2 & 98.2 & \textbf{98.2} & 98.1 & \textbf{98.2} & \textbf{0.14} & 1.10 & 1.25 \\
% 100 & \textbf{98.0} & 97.9 & 97.9 & \textbf{98.3} & 98.2 & \textbf{98.3} & \textbf{0.17} & 1.36 & 1.55 \\
% 120 & 98.0 & 98.0 & 98.0 & \textbf{98.4} & 98.2 & \textbf{98.4} & \textbf{0.21} & 1.63 & 1.88 \\
% 140 & 97.8 & 97.8 & 97.8 & \textbf{98.2} & 98.1 & 98.1 & \textbf{0.24} & 1.97 & 2.19 \\
% 160 & \textbf{98.2} & 98.1 & \textbf{98.2} & \textbf{98.1} & 97.4 & 97.9 & \textbf{0.29} & 2.28 & 2.53 \\
% 180 & 98.1 & 98.1 & 98.1 & 98.3 & \textbf{98.5} & 98.3 & \textbf{0.33} & 2.57 & 2.85 \\
% 200 & 98.1 & 98.1 & \cellcolor{yellow} \textbf{98.2} & \textbf{98.3} & 98.0 & \cellcolor{yellow} 98.2 & \textbf{0.37} & 2.83 & \cellcolor{yellow} 3.17 \\
% \bottomrule
% \end{tabular}}
% \end{table*}
